# Supplementary material for: Morphology of active deformable 3D droplets
Source: arXiv:2010.10427 ancillary file (2020-10-20)
Supplement: Supplementary file 1 [file SI.pdf]

# Supplementary Information:
# Morphology of active self-deforming droplets

Liam J. Ruske and Julia M. Yeomans
(Dated: October 20, 2020)

## I. SUPPLEMENTARY MOVIES

**Movie S1**: Disclination line dynamics (left panel) and surface alignment of the director field (right panel) in spherical active drops for extensile and contractile activity. Disclination line segments are shown as thick lines coloured by the characteristic twist angle $\beta$. Surface defects, shown as blue arrows on the right panel, are connected via disclination lines running through the bulk. The surface alignment is indicated by the colour bar, where orange (black) indicates in-plane (perpendicular) director alignment with respect to the interface. The distribution of surface angle $\cos(\theta)$ over the total surface area is shown in the upper right.

**Movie S2**: Example of a soft, extensile droplet with constant formation and retraction of protrusions. The movie displays disclination line dynamics (left panel), local mean curvature of the surface (middle panel) and surface alignment of the director field (right panel). Disclination line segments are shown as thick lines coloured by the characteristic twist angle $\beta$. Surface defects, shown as blue arrows on the right panel, are connected via disclination lines running through the bulk. The surface alignment is indicated by the colour bar, where orange (black) indicates in-plane (perpendicular) director alignment with respect to the interface.

**Movie S3**: Run-and-tumble motion of a contractile droplet. The centre-of-mass position of the droplet in the $xy$-plane is shown by the black line. The movie displays disclination line dynamics (left panel) and surface alignment of the director field (right panel). Disclination line segments are shown as thick lines coloured by the characteristic twist angle $\beta$. Surface defects, shown as blue arrows on the right panel, are connected via disclination lines running through the bulk. The surface alignment is indicated by the colour bar, where orange (black) indicates in-plane (perpendicular) director alignment with respect to the interface.

**Movie S4**: Example of a soft, contractile droplet with surface wrinkles and dimples. The movie displays disclination line dynamics (left panel), local mean curvature of the surface (middle panel) and surface alignment of the director field (right panel). Disclination line segments are shown as thick lines coloured by the characteristic twist angle $\beta$. Surface defects, shown as blue arrows on the right panel, are connected via disclination lines running through the bulk. The surface alignment is indicated by the colour bar, where orange (black) indicates in-plane (perpendicular) director alignment with respect to the interface. The second half of the movie shows a 3D view of a typical droplet snapshot. Here the left panel shows a semi-transparent drop with highlighted surface alignment and the right panel shows the relative local radius of the surface, with light yellow marking the position of elevations and red areas the position of dimples or depressions.

## II. SUPPLEMENTARY FIGURES

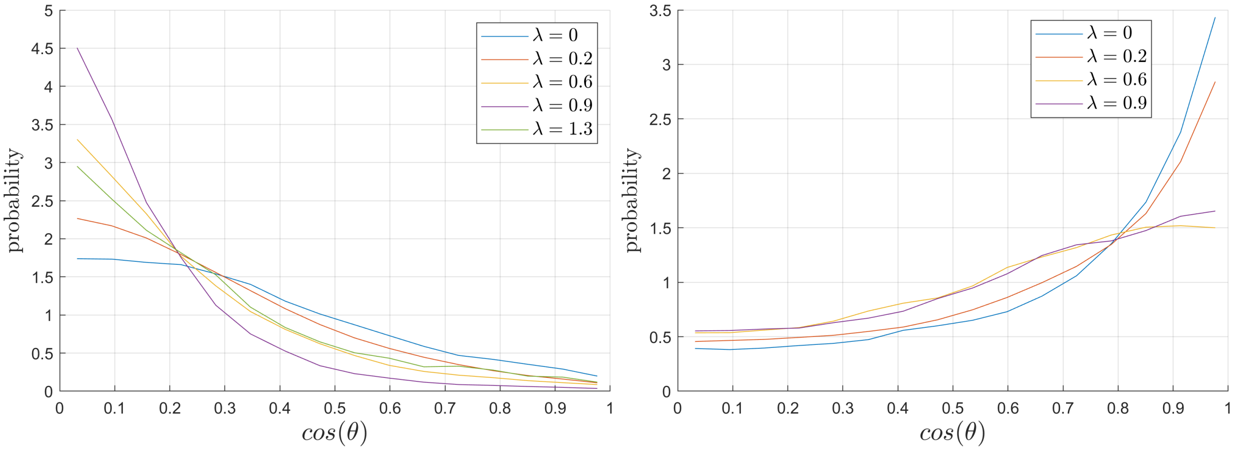


(a) Extensile activity $\zeta > 0$

(b) Contractile activity $\zeta < 0$

FIG. S1: Distribution of $\cos(\theta)$, where $\theta$ is the angle between the director and the surface normal, $0 \leq \theta < \pi/2$, for active droplets for different values of the flow-aligning parameter, $\lambda$. Extensile activity causes strong in-plane surface alignment ($\cos(\theta) \approx 0$) of the director with respect to the droplet's interface. Both flow-tumbling ($0 \leq \lambda < 1$) and flow-aligning ($\lambda > 1$) rod-like systems show strong active anchoring which is strongest roughly at the transition point $\lambda = 1$. Contractile activity leads to perpendicular surface alignment which is strongest for $\lambda = 0$ (spherical particles).

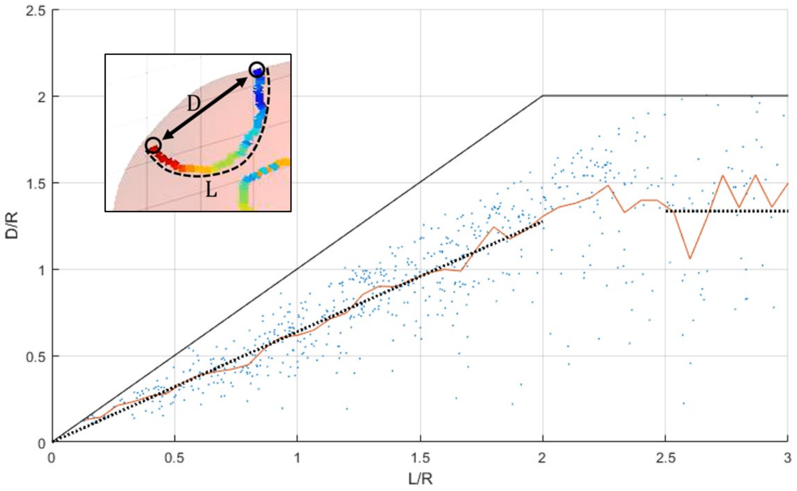


FIG. S2: The distance between endpoints (surface defects) of disclination lines $D$ first scales linearly with the total length of disclination lines before plateauing at a finite value. For disclination lines which are small compared to the droplet radios ($L < R$), the mean endpoint separation (orange line) scales as $D \approx 2/\pi L$ (black, dotted line). This shows that disclination lines mainly nucleate/annihilate at the droplet's surface and grow/shrink as half-circles. The endpoints of very long disclination lines ($L \gg R$) are randomly distributed over the droplet's surface so the mean separation of endpoints converges towards $D/R \approx 4/3$ (dashed, horizontal line). Individual observations are shown by blue dots.

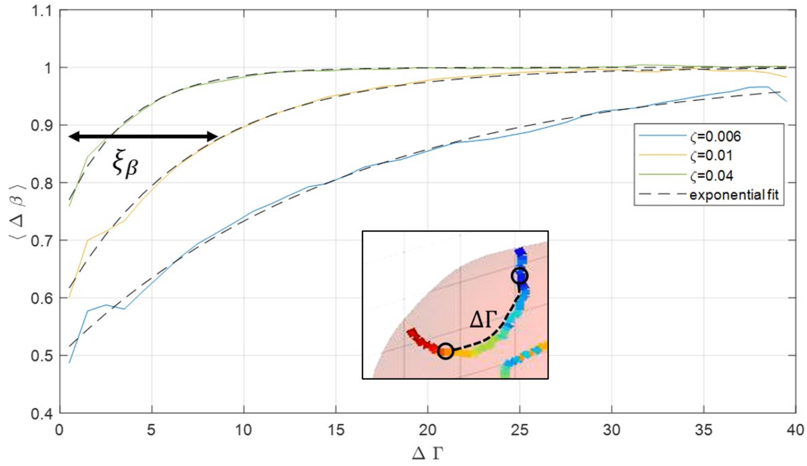


FIG. S3: Mean difference of local twist angle $\langle \Delta\beta \rangle$ between two points on the disclination line as a function of point separation $\Delta\Gamma$.

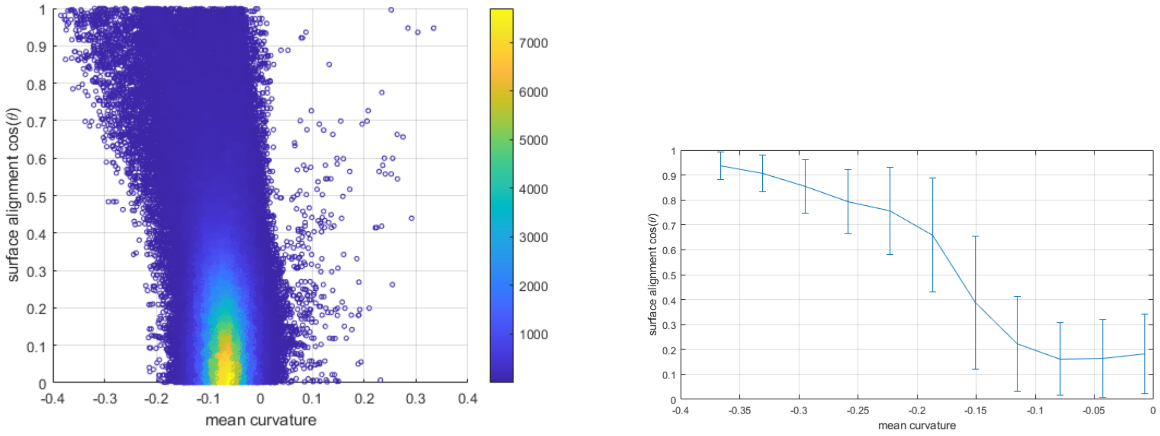


(a) Distribution of surface alignment $\cos(\theta)$ with local mean curvature of surface elements. The colorbar shows the density of data points.

(b) Mean surface alignment $\langle \cos(\theta) \rangle$ as a function of mean curvature. Error bars denote the standard deviation $\sqrt{Var(\cos(\theta))}$.

FIG. S4: In extensile droplets protrusions are formed by motile $\beta \approx \pi$ dislocation lines moving towards the interface. The director field inside protrusions is aligned along the protrusion axis, thereby introducing an area of perpendicular surface alignment at the ends of protrusions (points of large negative mean curvature). Surface alignment $\cos(\theta)$ is therefore correlated to mean surface curvature with perpendicular surface alignment ($\cos(\theta) \approx 1$) being associated with points of large negative curvature.

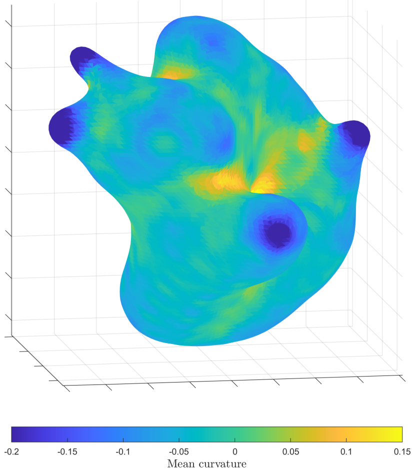


(a) Soft droplets form many protrusions extending into the surrounding medium. Colour coding shows the local mean curvature of the droplet surface.

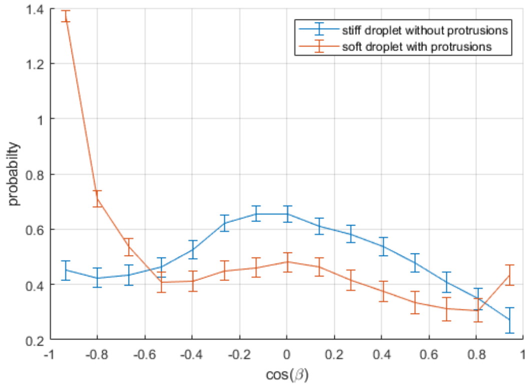


(b) Distribution of twist angle $\beta$ for disclination lines in stiff, spherical droplets and in soft droplets which form many protrusions.

FIG. S5: Protrusion formation relies on the presence of motile disclination lines pushing the interface outwards. After the initial formation of a bulge, the protrusion is pushed further outwards by almost straight $+1/2$ disclination lines as indicated by a sharp peak at $\beta \approx \pi$ in the probability distribution of the twist angle of disclination line segments.

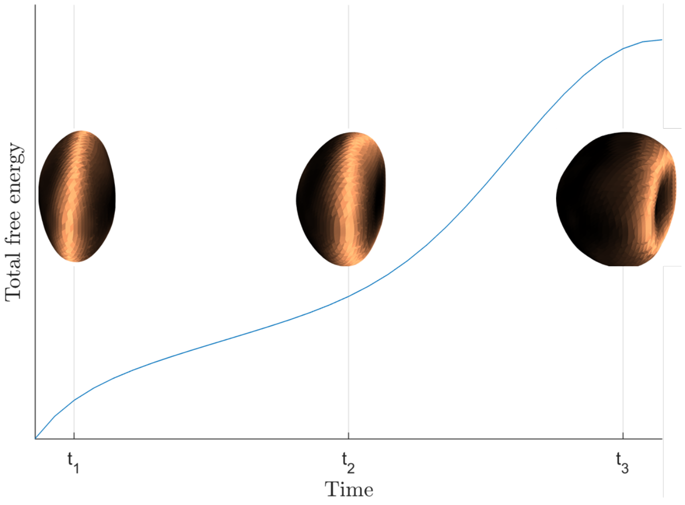


FIG. S6: Total free energy $\mathcal{F}$ as a function of time at different invagination stages $t_1 < t_2 < t_3$. Activity initially causes the formation of a bend-ring at the equator which contracts and moves towards one of the poles if active forces are sufficiently large to overcome the energy barrier associated with the contracting bend-ring. The exact droplet shapes and free energy profiles depend on model parameters such as the surface tensions, membrane rigidity, nematic elastic constant and bulk properties.

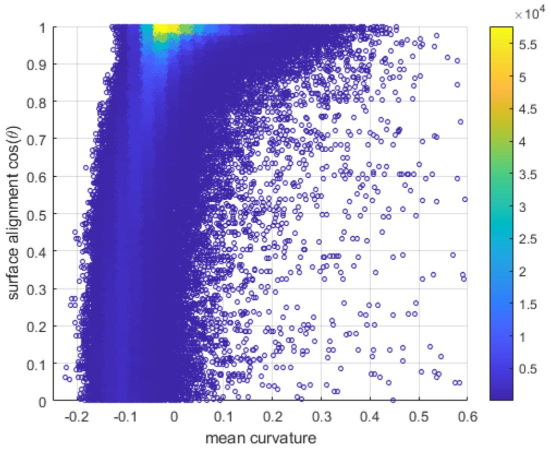


(a) Distribution of surface alignment $\cos(\theta)$ with local mean curvature of surface elements. The colorbar shows the density of data points.

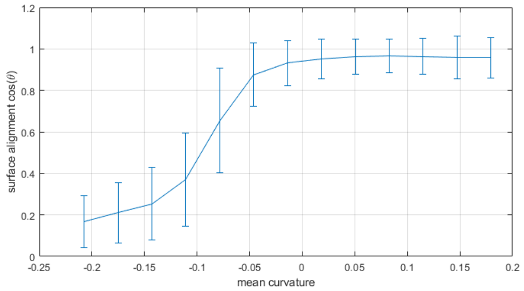


(b) Mean surface alignment $\langle\cos(\theta)\rangle$ as a function of mean curvature. Error bars denote the standard deviation $\sqrt{Var(\cos(\theta))}$.

FIG. S7: The surface of contractile droplets shows lines of in-plane surface alignment which forms stripe patterns. The in-plane alignment of the director field at the position of stripes is associated with nematic bend deformations in the bulk which push outwards and thus create comb-shaped deformations of the droplet. Surface alignment $\cos(\theta)$ is therefore correlated to local mean curvature with in-plane surface alignment ($\cos(\theta) \approx 0$) associated with points of large negative curvature.

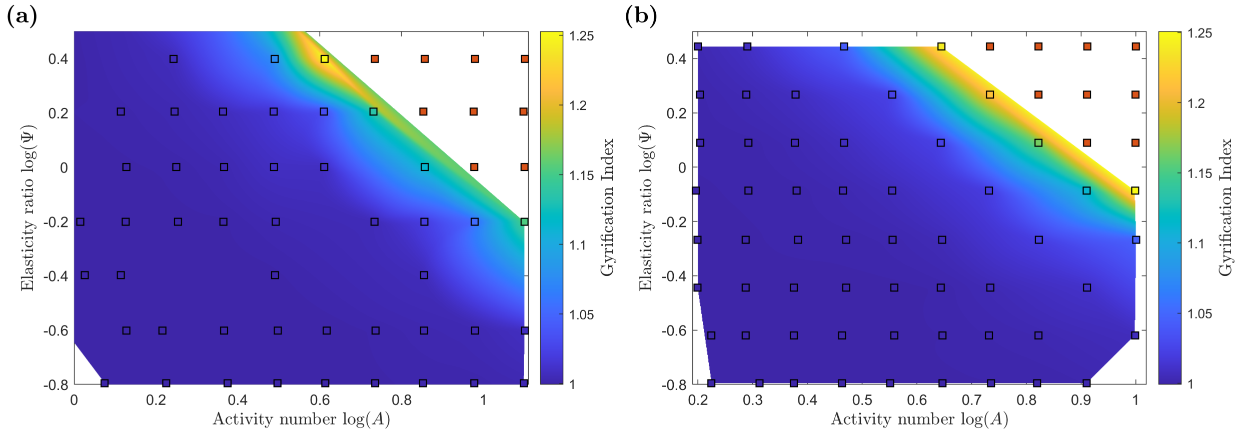


FIG. S8: Time-averaged gyrification index (GI) of droplets as a function of activity number $A$ and elastic constant to surface tension ratio $\Psi$ for extensile **(a)** and contractile activity **(b)**. The GI is defined as the ratio of surface area to the area of a spherical droplet and quantifies the strength of protrusion formation in extensile droplets **(a)** or the degree of wrinkling in contractile droplets **(b)**. It increases with both $A$ and $\Psi$ and reaches a maximum right before droplet break-up (orange squares).
